# Supplementary material for: Tight FPT Approximation for Constrained k-Center and k-Supplier
Source: arXiv:2110.14242 source file (2021-10-27)
Supplement: Supplementary file 1 [file Appendix_balanced_clustering_reduction.tex]

\section{Reduction for Balanced k-Supplier Problem}\label{appendix:reduction_balanced}

In this section, we show that the balanced $k$-supplier problem with cluster-wise constraints is easier than the balanced $k$-supplier problem with location-wise constraints. In other words, we show a polynomial time reduction from the balanced $k$-supplier problem with cluster-wise constraints to the balanced $k$-supplier problem with location-wise constraints. Formally, the two problems are defined as follows:

\begin{definition} [Balanced $k$-Supplier Problem with Cluster-Wise Constraints]
Given an instance $\mathcal{I} = (L,C,k,d,z,m)$ of the $k$-supplier problem and vectors $\ell,r \in \mathbb{Z}_{+}^{k}$, find a partitioning $\mathbb{O} = \{O_1,\dotsc,O_k\}$ of the client set $C$ that minimizes $\Psi^{*}(\mathbb{O})$ and satisfies that $\ell_{i} \leq |O_i| \leq r_{i}$ for every partition $O_{i} \in \mathbb{O}$.  
\end{definition}

\begin{definition} [Balanced $k$-Supplier Problem with Location-Wise Constraints]
Given an instance $\mathcal{I} = (L,C,k,d,z,m)$ of the $k$-supplier problem, a lower bound function $g \colon L \to \mathbb{Z}_{+}$, and an upper bound function $h \colon L \to \mathbb{Z}_{+}$, find a set $F$ of $k$ facility locations and assignment $\phi \colon C \to F$ that minimizes the assignment cost $\max_{x \in C}  \big\{ d(x,\phi(x))^{\zl} \big\}$ and satisfies that $g(f) \leq |\phi^{-1}(f)| \leq h(f)$ for every facility location $f \in F$.  
\end{definition}
\noindent We show the following theorem:

\begin{theorem}
Given any instance $\mathcal{I}_{C} = (L,C,k,d,z,m,\ell,r)$ of the balanced $k$-supplier problem with cluster-wise constraints, there is a polynomial time reduction to an instance $\mathcal{I}_{L} = (L',C,k,d,z,m,g,h)$ of the balanced $k$-supplier problem with location-wise constraints such that for any feasible solution $(\mathbb{O},F)$ of $\mathcal{I}_{C}$, there exists a feasible solution $(\phi,F')$ of $\mathcal{I}_{L}$ and vice-versa, such that the assignment cost $\Psi^{*}(F,\mathbb{O})$ is the same as the assignment cost: $\max_{x \in C}  \big\{ d(x,\phi(x))^{\zl} \big\}$.  
\end{theorem}

\begin{proof}
Given an instance $\mathcal{I}_{C} = (L,C,k,d,z,m,\ell,r)$ of the balanced $k$-supplier problem with cluster-wise constraints, we construct the instance $\mathcal{I}_{L}$ as follows. For every facility location $f \in L$, we create $k$ copies of $f$: $f^1,\dotsc,f^k$ such that $g(f^i) = \ell_{i}$ and $h(f^{i}) = r_i$ for every $f^i \in \{f^1,\dotsc,f^k\}$. We call this new facility set $L'$ and the new instance $\mathcal{I}_{L} = (L',C,k,d,z,m,g,h)$. This completes the reduction.

Let $(\mathbb{O},F)$ be any feasible solution of $\mathcal{I}_{C}$. That is, $\mathbb{O} = \{O_1,\dotsc,O_k\}$ is a partitioning of the client set $C$ such that $\ell_{i} \leq |O_{i}| \leq r_i$, and $F = \{f_1,\dotsc,f_k\}$ is a facility set such that $O_i$ is assigned to $f_i$. We define a feasible solution $(\phi,F')$ of $\mathcal{I}_{L}$ as follows. The facility set  is defined as $F' = \{f_{1}^{1},\dotsc, f_{k}^{k}\}$ and $\phi$ is defined such that all clients in $O_i$ are assigned to $f_{i}^{i}$. Since $f_{i}^{i}$ has $g(f_{i}^{i}) = \ell_{i}$ and $h(f_{i}^{i}) = r_{i}$, therefore, $g(f) \leq |\phi^{-1}(f)| \leq h(f)$ for every facility location $f \in F'$. Thus, $(\phi,F')$ is a feasible solution of $\mathcal{I}_{L}$. Furthermore, it is easy to see that the assignment cost does not change.

Similarly, let $(\phi,F')$ be any feasible solution of $\mathcal{I}_{L}$. That is, $\phi$ is an assignment of the client set $C$ to the facility set $F' \subseteq L'$ such that $g(f) \leq |\phi^{-1}(f)| \leq h(f)$ for every facility location $f \in F'$. We define a feasible solution $(\mathbb{O},F)$ as follows. The partition $O_i$ is defined as the set of clients assigned to that facility 

\end{proof}
